# Supplementary material for: Shortest Dominating Set Reconfiguration under Token Sliding
Source: arXiv:2307.10847 source file (2023-07-20)
Supplement: Supplementary file 1 [file appendix.tex]

\section{Fast matching on interval graphs}\label{app:fast_match}
This is a greedy algorithm that first tries to move a token to some match and otherwise to the right as much as possible.
The algorithm does not require the sets $D_s$ and $D_t$ to be dominating sets and supposes that the intersection is empty.
It keeps track of the tokens and matches them.
The algorithm describes processing of only token from $D_s$, processing token from $D_t$ is symmetric.

\begin{algorithm}[H]
  \caption{Fast matching between $D_s$ and $D_t$.}\label{alg:fast_match}
  \begin{algorithmic}[1]
    \Procedure{Match}{$G, D_s, D_t$}
      \For{$v$ ordered by $r(v)$}
        \If{$v \in D_s$}
          \State $X \gets \{ u | u \in N(v) \cap D_t \}$
          \If{$X \neq \emptyset$}
            \State $x \gets \min_{r(u)} X$
            \State $\Call{Match}{v,x}$
            \State $D_s \gets D_s \setminus \{v\}$
            \State $D_t \gets D_t \setminus \{x\}$
          \Else
            \State $w \gets \max_{r(u)} (\{ u | u \in N(v) \})$
            \State $D_s = \slide{D_s}{v}{w}$
          \EndIf
        \EndIf
      \EndFor
    \EndProcedure
  \end{algorithmic}
\end{algorithm}

\begin{lemma}\label{lemma:fast_match}
  Given $G$, an interval graph, and $D_s$, $D_t$ two multisets of the same size,
  \Cref{alg:fast_match} computes minimum matching in time $\calO(n\log n)$.
\end{lemma}
\begin{proof}
  We imagine that the tokens from $D_s$ or $D_t$ can move only to the right (if two tokens are matched, only the one more to the left moves to the right).
  First, we show that any token that can be immidiately matched is correctly matched greedily.
  Second, we argue that the token correctly moves as far as possible.

  Suppose that we have the token in $D_s$ at $v$ that has a neighbor from $D_t$ at $x$ with minimum $r(x)$
  and in all minimum matchings, $v$ cannot be matched to $x$.
  From all of these, we take the $v$ with least $r(v)$.
  We know then that both matches of $v$ and $x$ are to the right of $v$ (their right sides are).
  That means that if we match $v$ and $x$ and match of $v$ to match of $x$, the tokens have all possibilities of movements as $v$ and $x$.
  Therefore, they can match in the same number of steps as $v$ to match of $v$.
  Moreover, since $D_s$ and $D_t$ have empty intersection, the number of steps between $x$ and match of $x$ is at least $1$.
  
  Trivially, if we know that a token goes to the left, we can move it as much as possible.
  This justifies the choice of $w$.

  We traverse the graph once and for every vertex, we might need to look for neighbor with smallest (highest) $r(u)$, this can be done in time $\calO(\log n)$ by binary search.
  Which gives the time complexity $\calO(n\log n)$.
\end{proof}
